# Supplementary material for: Thermodynamics of Lithium Stripping and Limits for Fast Discharge in Lithium Metal Batteries
Source: arXiv:2103.03921 source file (2021-02-11)
Supplement: Supplementary file 1 [file Li_stripping_surf_SI.pdf]

# Supporting Information: Thermodynamics of Lithium Stripping and Limits for Fast Discharge in Lithium Metal Batteries

Victor Venturi[†] and Venkatasubramanian Viswanathan[*,†,‡]

†*Department of Mechanical Engineering, Carnegie Mellon University, Pittsburgh, Pennsylvania 15213, USA*

‡*Department of Physics, Carnegie Mellon University, Pittsburgh, Pennsylvania 15213, USA*

E-mail: venkvis@cmu.edu

# Computational details of interaction parameter estimation

In order to estimate the different regular solution parameters needed for our modeling, we used density functional theory (DFT), coupled with the Perdew, Burke, and Ernzerhof (PBE) exchange correlation functional[1] in the projector augmented wave (PAW) code GPAW.[2] The structures used were all slabs of at least 4 layers, with the bottom 2 layers kept fixed as to emulate bulk lithium, and can be seen in Figure S1. A 10 Åvacuum was applied, alongside a real-space grid spacing of 0.16 Åand a Monkhorst Pack scheme[3] sampling of the Brillouin zone with k-point density of 6 $Å^{-1}$. All calculations were converged to energy $< 0.5$ meV and force $< 0.05$ eV·$Å^{-1}$.

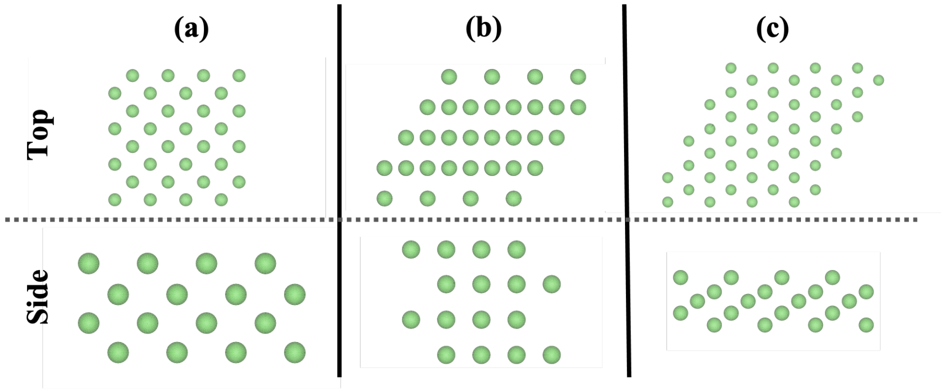


Figure S1: Top and side views of the structures used to calculate interaction parameters for the **(a)** (100), **(b)** (110), and **(c)** (111) surface facets. All structures had a minimum of 4 layers, and the bottom two layers of each structures were kept fixed to properly emulate bulk lithium.

To estimate the interaction parameters, systems with only one vacancy were created, allowing us to evaluate, for each facet, the value of $\epsilon_{VL}-\epsilon_{LL}$: the difference in energy between the pristine system and that with a vacancy is given by $E_{\text{single vacancy}}-E_{\text{pristine}} = z\,(\epsilon_{VL}-\epsilon_{LL})$. Next, by incorporating a second vacancy neighboring the first one, the value of $\epsilon_{VV}-\epsilon_{LL}$ can be estimated: $E_{\text{two vacancies}} - E_{\text{pristine}} = 2(z-1)\,(\epsilon_{VL}-\epsilon_{LL}) + (\epsilon_{VV}-\epsilon_{LL})$. Finally, to calculate the full interaction parameter we use

$$\Omega = \frac{z}{2}\left[2(\epsilon_{VL}-\epsilon_{LL}) - (\epsilon_{VV}-\epsilon_{LL})\right] = \frac{z}{2}(2\epsilon_{VL}-\epsilon_{VV}-\epsilon_{LL})$$

# References


(1) Perdew, J. P.; Burke, K.; Ernzerhof, M. Generalized Gradient Approximation Made Simple. *Phys Rev Lett* **1996**, *77*, 3865–3868, DOI: 10.1103/PhysRevLett.77.3865.

(2) Enkovaara, J.; Rostgaard, C.; Mortensen, J. J.; Chen, J.; Dułak, M.; Ferrighi, L.; Gavnholt, J.; Glinsvad, C.; Haikola, V.; Hansen, H., et al. Electronic structure calculations with GPAW: a real-space implementation of the projector augmented-wave method. *J Phys: Condens Matter* **2010**, *22*, 253202, DOI: 10.1088/0953-8984/22/25/253202.

(3) Monkhorst, H. J.; Pack, J. D. Special points for Brillouin-zone integrations. *Physical review B* **1976**, *13*, 5188.
